# Supplementary material for: Meta-node: A Concise Approach to Effectively Learn Complex Relationships in Heterogeneous Graphs
Source: arXiv:2210.14480 source file (2022-10-26)
Supplement: Supplementary file 1 [file 6-Supp.tex]

\newpage
% \onecolumn
\appendix
\section{Supplemental material}

\subsection{Implementation Details}
For comparison methods based on random-walk, we followed the settings of \cite{wang2021heco}.
Specifically, for metapath2vec, HERec, and HetGNN, the number of walks per node, the walk length, and the window size were set to $40, 100$, and $5$, respectively.
For GraphSAGE, GAE, DGI, metapath2vec, and HERec, the performances of all meta-path instances were measured and the best performance was reported.
For parameter settings other than those mentioned above, we followed the original setting of each paper.

\cite{glorot2010understanding} and used ADAM \cite{kingma2015adam} for optimization.
When conducting transformation of initial node features, Eq. (\ref{transform}), we applied batch normalization \cite{ioffe2015batch} before nonlinear activation.

Every experiments in this paper were conducted using a single Tesla T4 with 16GB memory.
Our code is implemented based Python version 3.7.11, Pytorch \cite{paszke2019pytorch} version 1.8.0, and PyTorch Geometric \cite{fey2019fast} version 2.0.1 which supports heterogeneous graph learning.
Models were optimized by ADAM \cite{kingma2015adam} for 10,000 epochs.
For nonlinear activation of each layer in the encoder, we used hyperbolic tangent function.
We present the hyper-parameter settings such as learning rate (lr), weight decay (wd), patience, dropout rate (r), dimension of learned representations (d), and number of layers in encoder (\#layers) of our method in Table ~\ref{tab:parameter}.
% For DBLP and ACM, we use same hyper-parameter settings for both node classification and node clustering tasks.
% For AMiner and Freebase, different hyper-parameters were used for node classification (cla.) and node clustering (clu.), respectively.
For node2vec, the number of walks per node, the walk length, and the window size are set to $10, 20$, and $10$, respectively for every dataset.

There do not exist features for `author', `subject' node types in ACM and every node type in AMiner and Freebase.
In these cases, some methods assign one-hot vectors as a unique node identifier for those types that do not have features. 
However, this one-hot vector strategy does not suitable for contrastive learning methods that generate negative samples by random permutation of features, including ours.
This is because a one-hot vector of negative samples can still serve as a unique node identifier after random permutations and cannot produce a useful supervising signal for contrastive learning.
Thus, we used node2vec \cite{grover2016node2vec} to extract the structural feature of each node that does not have features. 
The feature extraction is done after removing all information about the types of nodes and edges by transforming from a heterogeneous graph to a homogeneous graph.
Unlike some methods that apply message passing to the nodes of target node type only, we apply our MN-MPL to nodes of every type in the dataset.
% \begin{table*}[t]
%   \caption{The choices of hyper-parameters for each dataset.}
%   \vskip -0.1in
%   \label{tab:parameter}
%   \begin{tabular}{lcccccccc}
%     \toprule
%       Dataset & Learning rate & Weight decay & Patience & Dropout rate & Embedding dimension & \# of layers in encoder \\
%     \midrule
%     DBLP                      & 1e-2 & 1e-5 & 20  & 0.7 & 64  & 3 \\
%     ACM                       & 1e-2 & 1e-5 & 100 & 0.4 & 64  & 2 \\
%     AMiner (classification)   & 1e-3 & 0.0  & 50  & 0.9 & 500 & 1 \\
%     AMiner (clustering)       & 1e-3 & 0.0  & 50  & 0.7 & 500 & 1 \\
%     Freebase (classification) & 1e-3 & 0.0  & 50  & 0.7 & 800 & 1 \\
%     Freebase (clustering)     & 1e-4 & 1e-4 & 40  & 0.0 & 500 & 1 \\
%   \bottomrule
% \end{tabular}
% \end{table*}

% \begin{table}[h!]
%   \caption{The choices of hyper-parameters for each dataset.}
%   \label{tab:parameter}
%   \begin{tabular}{lcccccccc}
%     \toprule
%       Dataset & lr & wd & Patience & r & d & \#layers\\
%     \midrule
%     DBLP                      & 1e-2 & 1e-5 & 20  & 0.7 & 64  & 3 \\
%     ACM                       & 1e-2 & 1e-5 & 100 & 0.4 & 64  & 2 \\
%     AMiner (cla.)   & 1e-3 & 0.0  & 50  & 0.9 & 500 & 1 \\
%     AMiner (clu.)       & 1e-3 & 0.0  & 50  & 0.7 & 500 & 1 \\
%     Freebase (cla.) & 1e-3 & 0.0  & 50  & 0.7 & 800 & 1 \\
%     Freebase (clu.)     & 1e-4 & 1e-4 & 40  & 0.0 & 500 & 1 \\
%   \bottomrule
% \end{tabular}
% \end{table}

\begin{table}[h!]
\centering
  \caption{The choices of hyper-parameters for each dataset.}
  \label{tab:parameter}
  \resizebox{0.46\textwidth}{!}{\begin{tabular}{lcccccccc}
    \toprule
    Dataset   & lr   & wd   & Patience & r   & d   & \#layers\\
    \midrule
    DBLP       & 1e-2 & 1e-5 & 20       & 0.8 & 64  & 3 \\
    ACM        & 1e-2 & 1e-5 & 100      & 0.8 & 64  & 2 \\
    AMiner     & 1e-3 & 0.0  & 100      & 0.7 & 512 & 1 \\
    Freebase   & 1e-3 & 0.0  & 50       & 0.4 & 700 & 1 \\
  \bottomrule
\end{tabular}}
\end{table}
